# Supplementary material for: OpenTSLM TeeMoE: A Unified Time-Series Language Model for Forecasting, Contextual Prediction, and Reasoning
Source: arXiv:2609.40265 source file (2026-10-07)
Supplement: Supplementary file 1 [file recipe_format.tex]

\RequirePackage{framed}
\RequirePackage{needspace}
\newenvironment{recipebox}[1]{\par\addvspace{1em}\Needspace{7\baselineskip}
  \long\def\MidFrameCommand##1{\fboxrule=\FrameRule\fboxsep=\FrameSep
    \fbox{\vbox{\hbox{\strut\textbf{#1 (continued)}}\smallskip\hbox{##1}}}}\let\LastFrameCommand\MidFrameCommand
  \begin{framed}\textbf{#1}\par\smallskip
}{\end{framed}\par
}
\newcommand{\recipedivider}{\par\medskip\hrule\medskip
  \noindent\textbf{Training data}\par\smallskip
}
\newcommand{\recipedatarow}[2]{\textbullet\enspace #1 & #2\\}
\newenvironment{recipedatalist}{\begin{list}{\textbullet}{\setlength{\leftmargin}{1.2em}\setlength{\labelwidth}{0.7em}\setlength{\labelsep}{0.5em}\setlength{\itemsep}{1pt}\setlength{\parsep}{0pt}\setlength{\topsep}{2pt}}}{\end{list}}
\newcommand{\recipedataitem}[2]{\item #1\hfill\mbox{#2}}
